# Supplementary material for: Utilizing Graph Generation for Enhanced Domain Adaptive Object Detection
Source: arXiv:2406.06535 source file (2024-11-12)
Supplement: Supplementary file 1 [file 7_appendix.tex]

\clearpage
\appendix
\onecolumn

\section{Proof of Proposition~\ref{proposition_first} }
\label{proof1}
\textbf{Proposition 4.1}
\textit{
Define the first-order SNNs ODE as $\frac{d u_t^\tau}{d \tau}=g(u_t^\tau,\tau)$, and first-order Graph ODE as $\frac{d u_t^\tau}{d t}=f(u^{\tau}_t,t)$, then the first-order graph PDE network can be formulated as:
    \begin{equation}
        u_{t+1}^{\tau+1}=u_0^0+\int_0^T f\left(u^0_y+\int_0^N g(u_y^x,x)dx\right)dy+\int_0^N g\left(u_0^x+\int_0^{T-1} f(u_y^x,y)dy\right)dx.\nonumber
    \end{equation}}
\textit{Proof.}
\begin{equation}
    \frac{d u_t^\tau}{d \tau}=g(u_t^\tau,\tau), \quad \frac{d u_t^\tau}{d t}=f(u^{\tau}_t,t),\nonumber
\end{equation}
$u_t^\tau$ is a function related to variable $t$ and $\tau$, we have $\frac{\partial u_t^\tau}{\partial \tau}=g(u_t^\tau)$ and $\frac{\partial u_t^\tau}{\partial t}=f(u_t^\tau)$. Thus,
\begin{equation}
    u_t^{\tau+1}=u_t^\tau+\int_\tau^{\tau+1}g(u_t^x,x)dx,\;\;
u_{t+1}^{\tau+1}=u_t^{\tau+1}+\int_t^{t+1}f(u^{\tau+1}_y,y)dy,
    \end{equation}
\begin{equation}
\begin{aligned}
u_T^N=&u_{T-1}^{N-1}+\int_{T-1}^T f(u^N_y,y)dy+\int_{N-1}^N g(u_{T-1}^x,x)dx \\
=&u_{T-2}^{N-2}+\int_{T-2}^{T}f\left(u^{N}_y,y\right)dy+\int_{N-2}^{N}g(u_{T-1}^x,x)dx\\
=&u_0^0+\int_0^T f\left(u^{N}_y,y\right)dy+\int_0^N g(u_{T-1}^x,x)dx\\
=&u_0^0+\int_0^T f\left(u^{N-1}_y+\int_{N-1}^{N}g(u_y^x,x)dx\right)dy+\int_0^N g\left(u_{T-2}^x+\int_{T-2}^{T-1}f(u_y^x,y)dy\right)dx\\
=&u_0^0+\int_0^T f\left(u^0_y+\int_0^N g(u_y^x,x)dx\right)dy+\int_0^N g\left(u_0^x+\int_0^{T-1} f(u_y^x,y)dy\right)dx.\\
\end{aligned}
\end{equation}
By adding the initial state on each time step and latency with $u_t^0=0$ and $u_0^\tau=0$, we have:
\begin{equation}
\begin{aligned}
    u_T^N =& \int_0^T f\left(\int_0^N g(u_y^x,x)dx\right)dy+\int_0^N g\left(\int_0^{T-1} f(u_y^x,y)dy\right)dx\\
    =&\underbrace{\int_0^{T-1} f\left(\int_0^N g(u_y^x,x)dx\right)dy+\int_0^N g\left(\int_0^{T-1} f(u_y^x,y)dy\right)dx}_{first\;\; term}+\underbrace{\int_{T-1}^{T} f\left(\int_0^N g(u_y^x,x)dx\right)dy}_{second\;\; term}\\
    =&2\int_0^{T-1} f\left(\int_0^N g(u_y^x,x)dx\right)dy+\int_{T-1}^{T} f\left(\int_0^N g(u_y^x,x)dx\right)dy.
\end{aligned}
\end{equation}
The first term denotes that the SNNs and CGNNs are interactively updated during the time step $0$ to $T-1$, and the second term denotes that at the last time step $T$, \method{} simply calculates the CGNNs process while ignoring the SNNs for prediction.

\section{Proof of Eqn.~\ref{second_order_representation} }
\label{eqn12}

\textit{Proof.}
From Eq.~\ref{second_rep}, we have:
\begin{equation}
    u(\tau+1)=\beta^2u(\tau-k+1)+\alpha \sum_{i=0}^{k-1}\beta^iI_{syn}(\tau-i)+\sum_{i=0}^{k-1}\beta^i(I_{input}(\tau-i)-V_{th}s(\tau-i)),
\end{equation}
\begin{equation}
    u(N)=\alpha \sum_{n=0}^{N-1}\beta^n I_{syn}(N-n-1)+\sum_{n=0}^{N-1}\beta^n(I_{input}(N-n-1)-V_{th}s(N-n-1)).
\end{equation}
Due to:
\begin{equation}
    I_{syn}(\tau+1)=\alpha^k I_{syn}(\tau-k+1)+\sum_{i=0}^k \alpha^i I_{input}(\tau-i),
\end{equation}
we have,
\begin{equation}
\begin{aligned}
    u(N)=&\alpha \sum_{n=0}^{N-1}\beta^{N-n-1}I_{syn}(n)+\sum_{n=0}^{N-1}\beta^{N-n-1}\left(I_{input}(n)-V_{th}s(n)\right)\\
    =&\alpha \left(\left(\frac{\beta^{N-1}\alpha^{-1}\left(1-(\frac{\alpha}{\beta})^N\right)}{{1-\frac{\alpha}{\beta}}}\right)I_{in}(0)+\left(\frac{\beta^{N-2}\alpha^{-1}\left(1-(\frac{\alpha}{\beta})^{N-1}\right)}{{1-\frac{\alpha}{\beta}}}\right)I_{in}(1)+\cdots\right.\\ 
    &\left.+\left(\frac{\beta^{N-i}\alpha^{-1}\left(1-(\frac{\alpha}{\beta})^{N-i+1}\right)}{{1-\frac{\alpha}{\beta}}}\right)I_{in}(i-1)+\cdots+(\beta^2 \alpha^{-1}+\beta+\alpha)I_{in}(N-3)\right.\\
    &\left.+(\beta \alpha^{-1}+1)I_{in}(N-2)+\alpha^{-1}I_{in}(N-1)\right)-\sum_{n=0}^{N-1}\beta^{N-n-1}V_{th}s(n)\\
    =&\frac{1}{\beta-\alpha}\left(\left(\beta^N\left(1-\left(\frac{\alpha}{\beta}\right)^N\right)I_{in}(0)\right)+\dots+\left(\beta^{N-i+1}\left(1-\left(\frac{\alpha}{\beta}\right)^{N-i+1}\right)I_{in}(i-1)\right)\right.\\ 
    &\left.+\cdots+(\beta-\alpha)I_{in}(N-1)\right)-\sum_{n=0}^{N-1}\beta^{N-n-1}V_{th}s(n)\\
    =&\frac{1}{\beta-\alpha}\sum_{n=0}^{N-1}(\beta^{N-n}-\alpha^{N-n})I_{in}(n)-\sum_{n=0}^{N-1}\beta^{N-n-1}V_{th}s(n).\nonumber
\end{aligned}
\end{equation}

Define $\hat{I}(N)=\frac{1}{(\beta-\alpha)^2}\frac{\sum_{n=0}^{N-1}(\beta^{N-n}-\alpha^{N-n})I_{in}(n)}{\sum_{n=0}^{N-1}(\beta^{N-n}-\alpha^{N-n})}$, and $\hat{a}(N)=\frac{1}{\beta^2}\frac{V_{th}\sum_{n=0}^{N-1}\beta^{N-n}s(n)}{\sum_{n=0}^{N-1}(\beta^{N-n}-\alpha^{N-n})}$, we have:
\begin{equation}
    \hat{a}(N)=\frac{\beta-\alpha}{\beta}\frac{\hat{I}(N)}{\Delta \tau}-\frac{u(N)}{\Delta \tau\beta \sum_{n=0}^{N-1}(\beta^{N-n}-\alpha^{N-n})}\approx \frac{\tau_{syn}\tau_{mem}}{\tau_{mem}-\tau_{syn}}\hat{I}(N)-\frac{u(N)}{\Delta \tau\beta \sum_{n=0}^{N-1}(\beta^{N-n}-\alpha^{N-n})},\nonumber
\end{equation}
where $\alpha=exp(-\Delta \tau/\tau_{syn})$, $\beta=exp(-\Delta \tau/\tau_{mem})$.

\section{Proof of Proposition~\ref{proposition_third} }
\label{proof43}
\textbf{Proposition 4.3}
\textit{
    Define the second-order SNNs as $\frac{d^2u_t^\tau}{d\tau^2}+\delta \frac{du_t^\tau}{d\tau}=g(u^{\tau}_t,\tau)$, and second-order CGNNs as $\frac{d^2u_t^\tau}{dt^2}+\gamma \frac{du_t^\tau}{dt}=f(u^{\tau}_t,t)$, then the second-order \method{} is formulated as:
    \begin{equation}
        u_t^\tau=\int_{0}^T h\left(\int_0^N e(u_t^\tau)d\tau\right)dt=\int_0^N e\left(\int_0^T h(u_t^\tau)dt\right)d\tau,\nonumber
    \end{equation}
    \begin{equation}
        \frac{\partial^2 u_t^\tau}{\partial \tau^2}+\delta \frac{\partial u_t^\tau}{\partial \tau}=g(u_t^\tau),\quad \frac{\partial^2 u_t^\tau}{\partial t^2}+\gamma \frac{\partial u_t^\tau}{\partial t}=f(u_t^\tau),\nonumber
    \end{equation}}
where $e(u_t^\tau)=\int_0^N g(u_t^\tau)d\tau-\delta (u_t^N-u_t^0)$, and $h(u_t^\tau)=\int_0^T f(u_t^\tau)dt-\gamma (u_T^\tau-u_0^\tau)$.

\textit{Proof.}
Obviously,
\begin{equation}
    \frac{\partial^2 u_t^\tau}{\partial \tau^2}+\delta \frac{\partial u_t^\tau}{\partial \tau}=g(u_t^\tau),\quad \frac{\partial^2 u_t^\tau}{\partial t^2}+\gamma \frac{\partial u_t^\tau}{\partial t}=f(u_t^\tau),\nonumber
\end{equation}
\begin{equation}
    so,\quad \frac{\partial u_t^\tau}{\partial \tau}+\delta (u_t^N-u_t^0)=\int_0^N g(u_t^\tau)d\tau,\quad \frac{\partial u_t^\tau}{\partial t}+\gamma (u_T^\tau-u_0^\tau)=\int_0^T f(u_t^\tau)dt.\nonumber
\end{equation}
Define $e(u_t^\tau)=\int_0^N g(u_t^\tau)d\tau-\delta (u_t^N-u_t^0)$, and $h(u_t^\tau)=\int_0^T f(u_t^\tau)dt-\gamma (u_T^\tau-u_0^\tau)$, we have:
\begin{equation}
    \frac{\partial u_t^\tau}{\partial \tau}=e(u_t^\tau),\quad \frac{\partial u_t^\tau}{\partial t}=h(u_t^\tau),\nonumber
\end{equation}
thus,
\begin{equation}
    u_t^\tau=\int_{0}^T h\left(\int_0^N e(u_t^\tau)d\tau\right)dt=\int_0^N e\left(\int_0^T h(u_t^\tau)dt\right)d\tau,\nonumber
\end{equation}
where $\frac{\partial e(u_t^\tau)}{\partial \tau}=g(u_t^\tau)$ and $\frac{\partial h(u_t^\tau)}{\partial t}=f(u_t^\tau)$.

\section{Proof of Proposition~\ref{proposition_fourth}}
\label{proof44}
% \begin{proposition}
% \label{proposition_fourth}
\textbf{Proposition~\ref{proposition_fourth}}
   \textit{ Let $\mathbf{X}^n$ and $\mathbf{Y}^n$ be the node features, generated by Eqn.~\ref{second_graph_ode}, and $\Delta t \ll 1$. The gradient of the second-order CGNNs $\mathbf{W}_l$ is bounded as Eqn.~\ref{bound_gnn1}, and the gradient of the second-order SNNs $\mathbf{W}^k$ is bounded as Eqn.~\ref{bound_snn1}:}
    \begin{equation}
    \label{bound_gnn1}
    \begin{aligned}
        \left|\frac{\partial \mathcal{L}}{\partial \mathbf{W}_l}\right| \leq \frac{\beta^{'}\hat{\mathbf{D}}\Delta t (1+\Gamma T\Delta t)}{v}\left(\max\limits_{1\leq i \leq v} (|\mathbf{X}_i^0|+|\mathbf{Y}_i^0|)\right)+\frac{\beta^{'}\hat{\mathbf{D}}\Delta t (1+\Gamma T\Delta t)}{v}\left(\max\limits_{1\leq i \leq v}|\bar{\mathbf{X}_i}|+\beta \sqrt{T\Delta t}\right)^2,
    \end{aligned}
    \end{equation}
    \begin{equation}
    \label{bound_snn1}
    \begin{aligned}
    % \left|\frac{\partial \mathcal{L}}{\partial \mathbf{W}^k}\right|\leq
    \left|\frac{\partial \mathcal{L}}{\partial \mathbf{W}^k}\right| \leq \frac{(1+T\Gamma \Delta t)(1+N\Theta \Delta \tau)V_{th}}{v\beta^2 \Delta \tau}\left(\max\limits_{1\leq i \leq v}|\mathbf{X}_i^N|+\max\limits_{1\leq i \leq v}|\bar{\mathbf{X}}_i|\right).
    \end{aligned}
    \end{equation}
% \end{proposition}
where $
    \beta=\max\limits_x |\sigma(x)|$, $ \beta^{'}=\max\limits_x|\sigma^{'}(x)|$, $\hat{D}=\max\limits_{i,j\in\mathcal{V}}\frac{1}{\sqrt{d_id_j}}$, and $\Gamma:=6+4\beta^{'}\hat{D}\max\limits_{1\leq n\leq T}||\mathbf{W}^n||_1$, $\Theta:=6+4\beta^{'}\hat{D}\max\limits_{1\leq n\leq N}||\mathbf{W}^n||_1.$ $d_i$ is the degree of node $i$, $\mathbf{\bar{X}}_i$ is the label of node $i$.
    
\begin{equation}
\begin{aligned}
    \frac{\partial \mathcal{L}}{\partial \bm{W}^k}&=\frac{\partial \mathcal{L}}{\partial \bm{Z}_T^N} \frac{\partial \bm{Z}_T^N}{\partial \bm{Z}_l^N} \frac{\partial \bm{Z}_l^N}{\partial \bm{W}^k}=\frac{\partial \mathcal{L}}{\partial \bm{Z}_T^N}\prod_{n=l+1}^T\frac{\partial \bm{Z}_n^N}{\partial \bm{Z}_{n-1}^N}\frac{\partial \bm{Z}_l^N}{\partial \bm{W}^k}\\
    &=\frac{\partial \mathcal{L}}{\partial \bm{Z}_T^N}\prod_{n=l+1}^T\frac{\partial \bm{Z}_n^N}{\partial \bm{Z}_{n-1}^N} \frac{\partial \bm{Z}_l^N}{\partial \bm{Z}_l^k} \frac{\partial \bm{Z}_l^k}{\partial \bm{W}^k}\\
    &=\frac{\partial \mathcal{L}}{\partial \bm{Z}_T^N}\prod_{n=l+1}^T\frac{\partial \bm{Z}_n^N}{\partial \bm{Z}_{n-1}^N} \prod_{i={k+1}}^N\frac{\partial \bm{Z}_l^i}{\partial \bm{Z}_l^{i-1}} \frac{\partial \bm{Z}_l^k}{\partial \bm{W}^k},\nonumber
    % &=\frac{\partial \mathcal{L}}{\partial o_T^N} \prod_{n=l+1}^N\frac{\partial o_n^N}{\partial o_{n-1}^N} \sum_{\tau=1}^T\left(\frac{\partial \bm{o}_\tau^{l+1}}{\partial \bm{W}^l} + \sum_{k<\tau} \prod_{i=\tau-1}^k\left(\frac{\partial \bm{o}_{i+1}^{l+1}}{\partial \bm{o}_{i}^{l+1}}+\frac{\partial \bm{o}_{i+1}^{l+1}}{\partial \bm{s}_i^{l+1}}\frac{\partial \bm{s}_i^{l+1}}{\partial \bm{u}_i^{l+1}}\right)\frac{\partial \bm{u}_k^{l+1}}{\partial \bm{W}^l}\right)\\
    % &=\frac{\partial \mathcal{L}}{\partial u_T^N} \prod_{n=l+1}^N\frac{\partial u_n^N}{\partial u_{n-1}^N} \sum_{\tau=1}^T\left(\frac{\partial \bm{u}_\tau^{l+1}}{\partial \bm{W}^l} + \sum_{k<\tau} \prod_{i=\tau-1}^k\left(\frac{\partial \bm{u}_{i+1}^{l+1}}{\partial \bm{u}_{i}^{l+1}}\right)\frac{\partial \bm{u}_k^{l+1}}{\partial \bm{W}^l}\right)
\end{aligned}
\end{equation}
From~\cite{rusch2022graph}, we have:
\begin{equation}
\label{function_1}
    \left\lVert \frac{\partial \mathcal{L}}{\partial \bm{Z}_T^N} \right\rVert_{\infty}\leq \frac{1}{v}\left(\max\limits_{1\leq i \leq v}|\bm{X}_i^N|+\max\limits_{1\leq i \leq v}|\bar{\bm{X}}_i|\right), \quad \left\lVert\frac{\partial \bm{Z}_T^N}{\partial \bm{Z}_t^N}\right\rVert_\infty \leq 1+T\Gamma \Delta t.
\end{equation}
Due to the second-order SNN has a similar formulation to second-order GNN, we have a similar conclusion,
\begin{equation}
\label{function_2}
    \left\lVert\frac{\partial \bm{Z}_l^N}{\partial \bm{Z}_l^k}\right\rVert_\infty \leq 1+N\Theta \Delta \tau,
\end{equation}
with $\beta=\max\limits_x |\sigma(x)|$, $ \beta^{'}=\max\limits_x|\sigma^{'}(x)|$, $\hat{D}=\max\limits_{i,j\in\mathcal{V}}\frac{1}{\sqrt{d_id_j}}$, and $\Theta:=6+4\beta^{'}\hat{D}\max\limits_{1\leq n\leq N}||\bm{W}^n||_1.$, and with Eq.~\ref{back}, we have:
\begin{equation}
\label{function_3}
    \frac{\partial \bm{Z}_l^k}{\partial \bm{W}^k}\approx r(\bm{Z}_l^{k-1})\leq \frac{V_{th}}{\beta^2 \Delta \tau}.
\end{equation}

Multipling~\ref{function_1},~\ref{function_2} and~\ref{function_3}, we have the upper bound:
\begin{equation}
    \frac{\partial \mathcal{L}}{\partial \bm{W}^k}\leq \frac{(1+T\Gamma \Delta t)(1+N\Theta \Delta \tau)V_{th}}{v\beta^2 \Delta \tau}\left(\max\limits_{1\leq i \leq v}|\bm{X}_i^N|+\max\limits_{1\leq i \leq v}|\bar{\bm{X}}_i|\right).
\end{equation}
